# Supplementary material for: A thermally driven out-of-equilibrium two-impurity Kondo system
Source: arXiv:1806.10505 source file (2018-06-27)
Supplement: Supplementary file 1 [file Suplemental_Info.tex]

\documentclass[aps,twocolumn,superscriptaddress,showpacs]{revtex4-1}
\usepackage{amsmath,amssymb,multirow}
\usepackage{graphicx}
\usepackage{MnSymbol}
\usepackage[usenames]{color}
\begin{document}
\title{Suplemental information: A thermally driven out-of-equilibrium two-impurity Kondo system}
\author{Miguel A. Sierra}
\affiliation{Instituto de F\'{\i}sica Interdisciplinar y Sistemas Complejos
IFISC (UIB-CSIC), E-07122 Palma de Mallorca, Spain}
\author{Rosa L\'opez}
\affiliation{Instituto de F\'{\i}sica Interdisciplinar y Sistemas Complejos
IFISC (UIB-CSIC), E-07122 Palma de Mallorca, Spain}
\author{Jong Soo Lim}
\affiliation{School of Physics, Korea Institute for Advanced Study, Seoul 120-722, Korea}
\maketitle
\onecolumngrid
\section{Selfconsistent equations with $J=0$}\label{Sup:Eqs}

The value of the Kondo temperature and the positions of the Kondo peaks can be obtained using the condition of the unitary charge occupation $ b_{\alpha}^{\dag}b_{\alpha} + \sum_\sigma f_{\alpha \sigma}^{\dag}f_{\alpha \sigma}=1$ and the evolution of the bosonic operator $db_\alpha/dt=0$. The effect of the antiferromagnetic coupling $J$ gives an additional equation. However, we are interested in the $J=0$ case and the third equation will not be necessary.  In order to solve these equations we employ the nonequilibrium Green's function obtaining a new system of self-consistent equations
\begin{eqnarray}
\sum_\sigma G_{f\alpha\sigma,f\alpha\sigma}^<(t,t)&=&\frac{i}{\hbar}(1-N|b_\alpha|^2) \, , \label{Eq:GreenEq1}\\ 
\sum_\sigma {[g^r_{\alpha \sigma}]}^{-1}G^<_{f\alpha\sigma,f\alpha\sigma}(t,t)&=&-\frac{i}{\hbar}\lambda_\alpha N |b_\alpha|^2 \label{Eq:GreenEq2} \, , 
\end{eqnarray}
where $G^<_{f\alpha \sigma, f\alpha \sigma}$ is the nonequilibrium lesser Green's function of the quantum dot $\alpha$ with spin $\sigma=\pm 1/2$ and $g^r_{\alpha \sigma}$ is the equilibrium retarded Green's function of the dot $\alpha$.  After applying the Keldysh Green's function formalism and going to the Fourier space, equations \eqref{Eq:GreenEq1} and \eqref{Eq:GreenEq2} become
\begin{eqnarray}
\frac{2}{\pi}\int_{-\infty}^\infty d\omega \frac{\tilde{t}_\alpha\tilde{t}_{\bar{\alpha}} \tilde{\Gamma}_{\bar{\alpha}} f_{\bar{\alpha}}(\omega) +\tilde{\Gamma}_\alpha f_\alpha (\omega) [(\omega-\tilde{\varepsilon}_{\bar{\alpha}})^2+\tilde{\Gamma}_{\bar{\alpha}}^2]}{[(\omega -\tilde{\varepsilon}_{\alpha} +i\tilde{\Gamma}_\alpha)(\omega - \tilde{\varepsilon}_{\bar{\alpha}} +i\tilde{\Gamma}_{\bar{\alpha}}) - \tilde{t}_\alpha \tilde{t}_{\bar{\alpha}}][(\omega -\tilde{\varepsilon}_{\alpha} -i\tilde{\Gamma}_\alpha)(\omega - \tilde{\varepsilon}_{\bar{\alpha}} -i\tilde{\Gamma}_{\bar{\alpha}}) - \tilde{t}_\alpha \tilde{t}_{\bar{\alpha}}]}&=&(1-N\frac{\tilde{\Gamma}_{\alpha}}{\Gamma_\alpha}) \, ,\label{Eq:Eq1Int}  \\ 
\frac{2}{\pi}\int_{-\infty}^\infty d\omega \frac{(\omega-\tilde{\varepsilon}_{\alpha})(\tilde{t}_\alpha\tilde{t}_{\bar{\alpha}} \tilde{\Gamma}_{\bar{\alpha}} f_{\bar{\alpha}}(\omega) +\tilde{\Gamma}_\alpha f_\alpha (\omega) [(\omega-\tilde{\varepsilon}_{\bar{\alpha}})^2+\tilde{\Gamma}_{\bar{\alpha}}^2])}{[(\omega -\tilde{\varepsilon}_{\alpha} +i\tilde{\Gamma}_\alpha)(\omega - \tilde{\varepsilon}_{\bar{\alpha}} +i\tilde{\Gamma}_{\bar{\alpha}}) - \tilde{t}_\alpha \tilde{t}_{\bar{\alpha}}][(\omega -\tilde{\varepsilon}_{\alpha} -i\tilde{\Gamma}_\alpha)(\omega - \tilde{\varepsilon}_{\bar{\alpha}} -i\tilde{\Gamma}_{\bar{\alpha}}) - \tilde{t}_\alpha \tilde{t}_{\bar{\alpha}}]}&=&-(\varepsilon_\alpha -\tilde{\varepsilon}_\alpha) N \frac{\tilde{\Gamma}_{\alpha}}{\Gamma_\alpha} \, , \label{Eq:Eq2Int}
\end{eqnarray}
where we have redefined $\tilde{\Gamma}_\alpha = |b_\alpha|^2 \Gamma_\alpha$, $\tilde{\varepsilon}_\alpha = \varepsilon_\alpha+\lambda_\alpha$ and $\tilde{t}_\alpha = t |b_\alpha|^2 $ and $f_\alpha(\omega) = 1/(1+\exp{(\omega-\mu_\alpha)/k_BT_\alpha})$ is the Fermi distribution function of the reservoir $\alpha$ at a given electrochemical potential $\mu_\alpha$ and temperature gradient $T_\alpha$. The bar in $\bar{\alpha}$ indicates the opposite of the $\alpha$ reservoir (dot). We have to solve the integrals before performing the selfconsistent calculation. Therefore, we remark that the integrands have poles at
\begin{eqnarray}
\omega_{1,2}\equiv \omega_{\pm}&=&\frac{1}{2}\left(\tilde{\varepsilon}_\alpha - i\tilde{\Gamma}_\alpha	+\tilde{\varepsilon}_{\bar{\alpha}} - i\tilde{\Gamma}_{\bar{\alpha}} \pm \sqrt{(\tilde{\varepsilon}_\alpha-i\tilde{\Gamma}_\alpha-\tilde{\varepsilon}_{\bar{\alpha}}+i\tilde{\Gamma}_{\bar{\alpha}})^2+4|\tilde{t}|^2}\right) \, ,\\
\omega_{3,4}\equiv \omega_{\pm}^*&=&\frac{1}{2}\left(\tilde{\varepsilon}_\alpha + i\tilde{\Gamma}_\alpha	+\tilde{\varepsilon}_{\bar{\alpha}} + i\tilde{\Gamma}_{\bar{\alpha}} \pm \sqrt{(\tilde{\varepsilon}_\alpha+i\tilde{\Gamma}_\alpha-\tilde{\varepsilon}_{\bar{\alpha}}-i\tilde{\Gamma}_{\bar{\alpha}})^2+4|\tilde{t}|^2}\right) \, ,
\end{eqnarray}
where $|\tilde{t}|^2 = \tilde{t}_\alpha \tilde{t}_{\bar{\alpha}} = t^2 |b_\alpha|^2 |b_{\bar{\alpha}}|^2 $. Now, we are able to split the integrals into different terms of the form:
\begin{eqnarray}
J_\alpha(\omega_i) = \int_{-D}^D d\omega \frac{f_\alpha(\omega)}{\omega-\omega_i} \, , \label{Eq:Integral}
\end{eqnarray}
where $D$ is the bandwith of the system. After a lengthy calculation, equation \eqref{Eq:Integral} results
\begin{eqnarray}
J_\alpha(\omega_i) =\ln{\left|\frac{2\pi k_B T_\alpha}{D-\eta_i\omega_i}\right|}+\psi{\left(\frac{1}{2}-i\eta_i\frac{\omega_i-\mu_\alpha}{2\pi k_B T_\alpha}\right)}+\eta_i\frac{i\pi}{2} \, , \label{Eq:Integralsol}
\end{eqnarray}
where $\psi(x)$ denotes the digamma function and $\eta_i = \text{sgn} {({\text{Im}}[\omega_i])}$ is the sign of on the imaginary part of $\omega_i$. Adding \eqref{Eq:Integralsol} into Eqs. \eqref{Eq:Eq1Int} and \eqref{Eq:Eq2Int} we obtain the following solutions:
\begin{eqnarray}
\sum_{i} A_{i\alpha} J_\alpha(\omega_i)+B_{i\alpha} J_{\bar{\alpha}}(\omega_i)&=&\left(1-N\frac{\tilde{\Gamma}_{\alpha}}{\Gamma_\alpha}\right) \, , \label{Eq:Eq1sol}\\
\sum_{i} C_{i\alpha} J_\alpha(\omega_i)+D_{i\alpha} J_{\bar{\alpha}}(\omega_i)&=&-(\varepsilon_\alpha -\tilde{\varepsilon}_\alpha) N \frac{\tilde{\Gamma}_{\alpha}}{\Gamma_\alpha} \, , \label{Eq:Eq2sol}
\end{eqnarray}
where the coefficients are
\begin{eqnarray}
A_{i\alpha} &=& \frac{2}{\pi} \frac{\tilde{\Gamma}_\alpha [(\omega_i-\tilde{\varepsilon}_{\bar{\alpha}})^2+\tilde{\Gamma}_{\bar{\alpha}}^2]}{\prod_{j\neq i} (\omega_i-\omega_j)} \, ,\\
B_{i\alpha} &=& \frac{2}{\pi} \frac{|\tilde{t}|^2\tilde{\Gamma}_{\bar{\alpha}}}{\prod_{j\neq i} (\omega_i-\omega_j)} \, , \\
C_{i\alpha} &=& \frac{2}{\pi} \frac{\tilde{\Gamma}_\alpha[(\omega_i-\tilde{\varepsilon}_{\bar{\alpha}})^2+\tilde{\Gamma}_{\bar{\alpha}}^2] (\omega_i-\tilde{\varepsilon}_\alpha)}{\prod_{j\neq i} (\omega_i-\omega_j)} \, ,\\
D_{i\alpha} &=& \frac{2}{\pi} \frac{|\tilde{t}|^2\tilde{\Gamma}_{\bar{\alpha}}(\omega_i-\tilde{\varepsilon}_\alpha)}{\prod_{j\neq i} (\omega_i-\omega_j)}\, .
\end{eqnarray}
Once we obtain Eqs. \eqref{Eq:Eq1sol} and \eqref{Eq:Eq2sol}, we can proceed to solve numerically the system of equations. 
\section{Analytical solution of the currents}
The heat and electric currents are defined by the evolution of the hamiltonian and occupation operators of one of the reservoirs respectively,  
 \begin{eqnarray}
Q_\alpha&=& \frac{d}{dt}  \left(\sum_{k\sigma} \varepsilon_{\alpha k} c^\dagger_{\alpha k \sigma} c_{\alpha k \sigma}\right) -\frac{\mu_\alpha}{e} I_\alpha\; ,\\
 I_\alpha&=& -e \frac{d}{dt}  \left(\sum_{k\sigma} c^\dagger_{\alpha k \sigma} c_{\alpha k \sigma}\right) \;.
 \end{eqnarray} 
Using Keldysh nonequilibrium Green's function formalism, the current reads
\begin{eqnarray}
Q &=& \frac{1}{h} \int d\omega (f_L(\omega)- f_R(\omega)) (\omega-\mu_\alpha)\mathcal{T}(\omega) \, , \label{Eq:CurIntheat}\\
I &=& \frac{e}{h} \int d\omega (f_L(\omega)- f_R(\omega)) \mathcal{T}(\omega) \, , \label{Eq:CurInt}
\end{eqnarray}
with 
\begin{eqnarray}
\mathcal{T}(\omega)=4\sum_\sigma \tilde{\Gamma}_L \tilde{\Gamma}_R |G^r_{fL\sigma, fR\sigma}(\omega)|^2 \, . \label{Eq:TransGr} 
\end{eqnarray}
where $G^r_{fL\sigma, fR\sigma}(\omega)$ is the Fourier transform of the retarded Green's function $G^r_{fL\sigma, fR\sigma}(t,t')=-(i/\hbar)\theta(t-t')[\langle f_{L\sigma}(t) f_{R\sigma}(t') \rangle +\langle f_{R\sigma}(t') f_{L\sigma}(t) \rangle]$. Applying the equation-of-motion technique, we obtain the solution of the retarded Green's function,
\begin{eqnarray}
\mathcal{T}(\omega)=4\sum_\sigma \frac{\tilde{\Gamma}_L \tilde{\Gamma}_R |\tilde{t}|^2}{[(\omega -\tilde{\varepsilon}_{\alpha} +i\tilde{\Gamma}_\alpha)(\omega - \tilde{\varepsilon}_{\bar{\alpha}} +i\tilde{\Gamma}_{\bar{\alpha}}) - \tilde{t}_\alpha \tilde{t}_{\bar{\alpha}}][(\omega -\tilde{\varepsilon}_{\alpha} -i\tilde{\Gamma}_\alpha)(\omega - \tilde{\varepsilon}_{\bar{\alpha}} -i\tilde{\Gamma}_{\bar{\alpha}}) - \tilde{t}_\alpha \tilde{t}_{\bar{\alpha}}]}  \, . \label{Eq:TransInt} 
\end{eqnarray}
We notice that the integral of the current \eqref{Eq:CurInt} with the transmission \eqref{Eq:TransInt} has the same poles as the previous section yielding to a similar procedure. Using the solution of the integral in Eq. \eqref{Eq:Integralsol}, the currents become
\begin{eqnarray}
Q&=&\sum_i F_i \left[\psi{\left(\frac{1}{2}- i \eta_i\frac{\omega_i-\mu_L}{2\pi k_B T_L}\right)}-\psi{\left(\frac{1}{2}- i\eta_i\frac{\omega_i-\mu_R}{2\pi k_B T_R}\right)}\right] \, ,\\
I&=&\sum_i G_i \left[\psi{\left(\frac{1}{2}- i \eta_i\frac{\omega_i-\mu_L}{2\pi k_B T_L}\right)}-\psi{\left(\frac{1}{2}- i\eta_i\frac{\omega_i-\mu_R}{2\pi k_B T_R}\right)}\right] \, ,
\end{eqnarray}
where $\eta_i$ indicates the sign of the imaginary part of $\omega_i$ and 
\begin{eqnarray}
F_i &=& \frac{8}{h} \frac{\tilde{\Gamma}_L\tilde{\Gamma}_R |\tilde{t}|^2 (\omega_i-\mu_\alpha)}{\prod_{j\neq i} (\omega_i-\omega_j)} \, ,\\
G_i &=& \frac{8e}{h} \frac{\tilde{\Gamma}_L\tilde{\Gamma}_R |\tilde{t}|^2}{\prod_{j\neq i} (\omega_i-\omega_j)} \, .
\end{eqnarray}

\end{document}
